# Supplementary material for: Programmable large-scale simulation of bosonic transport in optical synthetic frequency lattices
Source: arXiv:2208.05088 source file (2022-08-10)
Supplement: Supplementary file 1 [file appendices.tex]

\section{Some appendix section}
\fromplm{TODO}
